# Supplementary material for: TAVA: Template-free Animatable Volumetric Actors
Source: arXiv:2206.08929 source file (2022-06-21)
Supplement: Supplementary file 1 [file eccv2022suppl.tex]

% updated April 2002 by Antje Endemann
% Based on CVPR 07 and LNCS, with modifications by DAF, AZ and elle, 2008 and AA, 2010, and CC, 2011; TT, 2014; AAS, 2016; AAS, 2020; TH, 2022

\documentclass[runningheads]{llncs}
\usepackage{graphicx}
% DO NOT USE \usepackage{times}, it will be removed by typesetters
%\usepackage{times}

\usepackage{tikz}
\usepackage{comment}
\usepackage{amsmath,amssymb} % define this before the line numbering.
\usepackage{color}
\usepackage[symbol]{footmisc}

\usepackage{booktabs}
\usepackage{adjustbox}
\usepackage{hyperref}
\hypersetup{
  colorlinks   = true, %Colours links instead of ugly boxes
  urlcolor     = red, %Colour for external hyperlinks
  linkcolor    = blue, %Colour of internal links
  citecolor   = green %Colour of citations, could be ``red''
}

\usepackage{bm}
\usepackage{pifont}
\usepackage{xcolor}
\usepackage{array}
\usepackage{microtype}
\usepackage{wrapfig}

\newcolumntype{P}[1]{>{\centering\arraybackslash}p{#1}} %% horizontal centering
\newcolumntype{M}[1]{>{\centering\arraybackslash}m{#1}} %% vertical centering

\newcommand\blfootnote[1]{%
  \begingroup
  \renewcommand\thefootnote{}\footnote{#1}%
  \addtocounter{footnote}{-1}%
  \endgroup
}

% The "axessiblity" package can be found at: https://ctan.org/pkg/axessibility?lang=en
\usepackage[accsupp]{axessibility}  % Improves PDF readability for those with disabilities.

% INITIAL SUBMISSION - The following two lines are NOT commented
% CAMERA READY - Comment OUT the following two lines
%\usepackage{ruler}
\usepackage[width=122mm,left=12mm,paperwidth=146mm,height=193mm,top=12mm,paperheight=217mm]{geometry}

\begin{document}
% \renewcommand\thelinenumber{\color[rgb]{0.2,0.5,0.8}\normalfont\sffamily\scriptsize\arabic{linenumber}\color[rgb]{0,0,0}}
% \renewcommand\makeLineNumber {\hss\thelinenumber\ \hspace{6mm} \rlap{\hskip\textwidth\ \hspace{6.5mm}\thelinenumber}}
% \linenumbers
\pagestyle{headings}
\mainmatter
\def\ECCVSubNumber{3781}  % Insert your submission number here

\title{Supplemental Materials for \\ TAVA: Template-free Animatable \\ Volumetric Actors} % Replace with your title

% INITIAL SUBMISSION 
% \begin{comment}
\titlerunning{ECCV-22 submission ID \ECCVSubNumber} 
\authorrunning{ECCV-22 submission ID \ECCVSubNumber} 
\author{Anonymous ECCV submission}
\institute{Paper ID \ECCVSubNumber}
% \end{comment}
%******************

% CAMERA READY SUBMISSION
\begin{comment}

\titlerunning{TAVA: Template-free Animatable Volumetric Actors}
% If the paper title is too long for the running head, you can set
% an abbreviated paper title here
%
\author{Ruilong Li$^{*,\dagger,||}$, Julian Tanke$^{+,\dagger,||}$, Minh Vo$^\dagger$, Michael Zollh\"ofer$^\dagger$,\\J\"urgen Gall$^+$, Angjoo Kanazawa$^{*}$, Christoph Lassner$^\dagger$}
\institute{\blfootnote{$^{||}$Work was done partially while Ruilong and Julian were interning at RLR.}$^*$UC Berkeley, $^+$University of Bonn, $^\dagger$Meta Reality Labs Research}
%
\authorrunning{Li et al.}
% First names are abbreviated in the running head.
% If there are more than two authors, 'et al.' is used.
%
%\institute{Princeton University, Princeton NJ 08544, USA \and
%Springer Heidelberg, Tiergartenstr. 17, 69121 Heidelberg, Germany
%\email{lncs@springer.com}\\
%\url{http://www.springer.com/gp/computer-science/lncs} \and
%ABC Institute, Rupert-Karls-University Heidelberg, Heidelberg, Germany\\
%\email{\{abc,lncs\}@uni-heidelberg.de}}
\end{comment}
%******************
\maketitle
\vspace*{-2em}

\input{suppl/main}

\clearpage
% ---- Bibliography ----
%
% BibTeX users should specify bibliography style 'splncs04'.
% References will then be sorted and formatted in the correct style.
%
\bibliographystyle{splncs04}
\bibliography{egbib}
\end{document}
